# Supplementary material for: Self-Supervised Meta-Learning for Few-Shot Natural Language Classification Tasks
Source: arXiv:2009.08445 source file (2020-11-15)
Supplement: Supplementary file 1 [file finetune.tex]

\begin{table}[t!]
\centering
% \resizebox{\linewidth}{!}{%
% \scalebox{0.57}{
\begin{tabular}{cc}
\Xhline{2\arrayrulewidth}
% \multicolumn{16}{c}{\textbf{Natural Language Inference}}                                              \\ \Xhline{2\arrayrulewidth}
% \multicolumn{1}{l}{} & \multicolumn{5}{c}{\textbf{MNLI}}              & \multicolumn{5}{c}{\textbf{QNLI}}               & \multicolumn{5}{c}{\textbf{RTE}}               \\ 
Hyper-parameter & MT-BERT  \\ \Xhline{2\arrayrulewidth}
% Activation Function & [ReLU, GeLU] \\ 
Tasks per batch & 4 \\ 
Support samples per task & 80\\ 
Query samples per task & 10\\ 
Number of classes in SSLMT & [2,3,4] \\ 
$d$ & 256  \\ 
Attention dropout & 0.1 \\ 
Hidden Layer Dropout & 0.1\\ 
% Inner Loop Learning Rate & --- & --- & --- & Meta-SGD (per-layer)\\ 
% Min Adapted Layer ($\nu$) & [0, 5, 8, 10, 11] & --- & --- & 0\\ 
Outer Loop Learning Rate & 1e-05\\ 
Adaptation Steps ($G$) & 7\\ 
$\lambda$ & 0.5\\ 
Meta-training Epochs & 1 \\
% Pooled Output & [True, False] \\ 
% Top layer [CLS] dropout & [0.45, 0.4, 0.3, 0.2, 0.1] & 0.1 & 0.2 & 0.1 \\ 
% Train Word Embeddings(Inner Loop) & [True, False] & --- & --- & True\\ 
% Use Pooled Output & [True , False] \\ 
% Data Sampling & [Square Root, Uniform] &Square Root & Square Root & Square Root \\ 
Lowercase text & False \\ 
Sequence Lenght & 128 \\ 
Warmup-ratio & 0.1 \\
\Xhline{2\arrayrulewidth}
\end{tabular}
% }
\caption{Hyper-parameters.}
\label{tab:params_our}
\end{table}
